# Supplementary material for: MDMMT: Multidomain Multimodal Transformer for Video Retrieval
Source: arXiv:2103.10699 source file (2021-03-19)
Supplement: Supplementary file 1 [file sect_appendix_isect_ytvid.tex]

In Tab.~\ref{tab:ytvid_isect} we report intersection by YouTube ID between test parts of MSRVTT(full, 1k-A, 1k-B) and ActivityNet with
train parts of MSRVTT(full, 1k-A, 1k-B), ActivityNet, Kinetics700, YouCook2, HowTo100m, MSVD.

\begin{table}[H]
	\centering
	\begin{tabular}{
			|@{\hspace{0.5\tabcolsep}}
			c@{\hspace{0.5\tabcolsep}}
			|@{\hspace{0.5\tabcolsep}}
			c@{\hspace{1\tabcolsep}}
			c@{\hspace{0.5\tabcolsep}}
			|@{\hspace{0.5\tabcolsep}}
			c@{\hspace{1\tabcolsep}}
			c@{\hspace{0.5\tabcolsep}}
			|@{\hspace{0.5\tabcolsep}}
			c@{\hspace{1\tabcolsep}}
			c@{\hspace{0.5\tabcolsep}}
			|@{\hspace{0.5\tabcolsep}}
			c@{\hspace{1\tabcolsep}}
			c@{\hspace{0.5\tabcolsep}}
			|
		}
		\toprule
		%\multirow{2}{*}{dataset}      &
		data &
		\multicolumn{2}{c|@{\hspace{0.5\tabcolsep}}}{M} &
		\multicolumn{2}{c|@{\hspace{0.5\tabcolsep}}}{M$_{\text{1k-a}}$} &
		\multicolumn{2}{c|@{\hspace{0.5\tabcolsep}}}{M$_{\text{1k-b}}$} &
		\multicolumn{2}{c|}{A}
		\\
		set &
		{\footnotesize test} & {\footnotesize train} & 
		{\footnotesize test} & {\footnotesize train} & 
		{\footnotesize test} & {\footnotesize train} &
		{\footnotesize test} & {\footnotesize train}
		\\
		\midrule
		M          	       & 0&0 & 0&0  & 104&179 & 2&4     \\
		M$_{\text{1k-a}}$  & 2362&1990  & 372&415 & 827&1007 & 2&4     \\ 
		M$_{\text{1k-b}}$  & 1689&1367  & 563&634 & 380&407  & 2&4     \\
		A	    	       & 0&0        & 0&0     & 0&0      & 0&0     \\
		K        		   & 5&4        & 1&1     & 0&0      & 408&408 \\
		Y       		   & 8&4        & 2&2     & 2&2      & 3&3     \\
		HT100M   		   & 147&117    & 39&38   & 57&53    & 175&175 \\
		MSVD		       & 3&1        & 2&1     & 0&0      & 1&1     \\
		\bottomrule
	\end{tabular}

	\caption{First stage. The leftmost column represents train parts of datasets, and the upper row represents test parts of datasets. Column "test" represents
	number of video segments in test part that have corresponding video in train part with the same YouTube ID. Column "train" represents number of video
	in train part that have corresponding pair in test part with the same ID. For example: if we combine M and YouCook2, we should remove 4 video from YouCook2 train.}
	\label{tab:ytvid_isect}
\end{table}

It is worth mention that MSRVTT 1k-A test and 1k-B test have a large overlap ratio by the YouTube ID with 1k-A train and 1k-B train correspondingly. 
Both splits have the overlap ratio of about 38\% between train part and test part.
We also emphasize that original MSRVTT full split does not have overlap by the YouTube ID between the test and train parts.

\begin{table}[H]
	\centering
	\begin{tabular}{
			|
			c
			|@{\hspace{0.5\tabcolsep}}
			c@{\hspace{0.5\tabcolsep}}
			c@{\hspace{0.5\tabcolsep}}
			c@{\hspace{0.5\tabcolsep}}
			|@{\hspace{0.5\tabcolsep}}
			c@{\hspace{0.5\tabcolsep}}
			c@{\hspace{0.5\tabcolsep}}
			c@{\hspace{0.5\tabcolsep}}
			|@{\hspace{0.5\tabcolsep}}
			c@{\hspace{0.5\tabcolsep}}
			c@{\hspace{0.5\tabcolsep}}
			c@{\hspace{0.5\tabcolsep}}
			|
		}
		\toprule
			%\multirow{2}{*}{dataset} &
			data &
			\multicolumn{3}{c| @{\hspace{0.5\tabcolsep}}}{M} & 
			\multicolumn{3}{c| @{\hspace{0.5\tabcolsep}}}{A} & 
			\multicolumn{3}{c|}{L}
			\\
		set &  
		{\footnotesize seen} &
		{\footnotesize found} &
		{\footnotesize total} & 
		{\footnotesize seen} &
		{\footnotesize found} &
		{\footnotesize total} & 
		{\footnotesize seen} &
		{\footnotesize found} &
		{\footnotesize total}
		\\
		\midrule
			M             & 10k&114&114 &    1k&      6&6 &   1k&0&0 \\ 
			A             & 10k&10&10   &    15k& 127&142 &   1k&0&0 \\
			L             & 3k& 6&6     &    2k&      0&0 &   ---&---&--- \\
			Y             & 2k& 13&13   &    1k&      7&7 &   1k&0&0 \\
			MSVD          & 1k& 1&1     &    1k&      1&1 &   1k&1&1 \\
			T             & 2k& 6&6     &    2k&      0&0 &   3k&0&0 \\
			V             & 2k& 3&3     &    0k&      0&0 &   1k&0&0 \\
			K             & 2k& 1&2     &    30k& 227&539 &   2k&0&0 \\
			HT100M        & 5k& 15&320  &    ---& ---&--- &   ---&---&--- \\
		\bottomrule
	\end{tabular}
	
	\caption{Second stage. The leftmost column represents train parts of datasets, and the upper row represents test parts of datasets.
			 Column "seen" represents number of video segments that we manually assess for given pair of datasets.
	         Column "found" represents the number of video in test part for which exists corresponding duplicate video segment in train part.
			 Column "total" represents an approximately estimated total number of videos from the test part that have a duplicate pair in the train part.
			 Symbol --- means that intersection is not computed because it requires too much human resources.}
	\label{tab:manual_isect_Ntest}
\end{table}

In Tab.~\ref{tab:manual_isect_Ntest} we report statistics for the second deduplication stage (searching by embeddings).
We did not compute an intersection for MSRVTT 1k-A and 1k-B splits. 

In this table we present number of manually found duplicates and estimated maximum number of duplicates for given pair of datasets. In most cases we managed to
find almost whole pairs.

Maximum number of duplicates is computed based on search curve $F(X)$. As we told in Sec.~\ref{ssec:how_many_pairs} search curve significantly depends on data. We compute
search curve for all pairs of datasets in Tab.~\ref{tab:manual_isect_Ntest}. The search curve for each particular pair of datasets is build exactly in the same way
as described in Sec.~\ref{ssec:how_many_pairs}. For example, to compute search curve for MSRVTT test and ActivityNet train we define MSRVTT test as $Q$, ActivityNet train as $G$, then augment
$Q$ to produce $\hat{Q}$, and use algorithm described in Sec.~\ref{ssec:how_many_pairs}.

Using column seen from Tab.~\ref{tab:manual_isect_Ntest} we can compute how many pairs need to be assessed to find full overlap between datasets. For example, we seen
5k pairs for HowTo100M dataset and MSRVTT (see row HT100M and column M), we found 15 duplicates, approximate maximum number of duplicates is 320: 5k * (320 / 15) = 106k.
So, to find full overlap with current version of algorithm it is needed to manually assess 106k video pairs, it is too much, that's why we did not found full intersection
for this pair of datasets.
